# Supplementary material for: Zero-Shot Audio-Visual Editing via Cross-Modal Delta Denoising
Source: arXiv:2503.20782 source file (2025-03-26)
Supplement: Supplementary file 1 [file dataset_table.tex]

\onecolumn
\begin{longtable}{p{3.5cm}p{7cm}ll}
\caption{Full Dataset Overview}
\label{tab:full_dataset}\\
\toprule
                                  YouTube ID and Time &                                        Source (top) and Target (bottom) Prompt  & Source Category &  Target Category\\
\midrule
\endfirsthead
\caption[]{Full Dataset Overview} \\
\toprule
                                  YouTube ID and Time &                                        Source (top) and Target (bottom) Prompt  & Source Category &  Target Category \\
\midrule
\endhead
\midrule
\multicolumn{4}{r}{{Continued on next page}} \\
\midrule
\endfoot

\bottomrule
\endlastfoot
  \multirow{2}{*}{MkJuGDph-1k\_000070} &                           a dog is barking&          dog &          lion \\
                                       &                          a lion is roaring&              &               \\
  \multirow{2}{*}{2jIv5qBTS88\_000009} &                           a dog is barking&          dog &          lion \\
                                       &                          a lion is roaring&              &               \\
 \multirow{2}{*}{3LO8iqmX\_LM\_000030} &                           a dog is barking&          dog &          lion \\
                                       &                          a lion is roaring&              &               \\
 \multirow{2}{*}{5nAvo9b2\_SY\_000020} &                           a dog is barking&          dog &          lion \\
                                       &                          a lion is roaring&              &               \\
  \multirow{2}{*}{21vfIdV2B60\_000030} &                           a dog is barking&          dog &          lion \\
                                       &                          a lion is roaring&              &               \\
  \multirow{2}{*}{92vVMZ4Zkcc\_000000} &                           a dog is barking&          dog &          lion \\
                                       &                          a lion is roaring&              &               \\
  \multirow{2}{*}{AyRHwZyYxEs\_000003} &                           a dog is barking&          dog &          lion \\
                                       &                          a lion is roaring&              &               \\
  \multirow{2}{*}{BCcdatk468s\_000070} &                           a dog is barking&          dog &          lion \\
                                       &                          a lion is roaring&              &               \\
  \multirow{2}{*}{CM5W31FRa7o\_000030} &                           a dog is barking&          dog &          lion \\
                                       &                          a lion is roaring&              &               \\
 \multirow{2}{*}{cRt6\_axWZqY\_000020} &                           a dog is barking&          dog &          lion \\
                                       &                          a lion is roaring&              &               \\
  \multirow{2}{*}{3d4Q9iU5Je8\_000006} &                           a cat is meowing&          cat &           dog \\
                                       &                           a dog is barking&              &               \\
 \multirow{2}{*}{3gjF-cVb\_m4\_000030} &                           a cat is meowing&          cat &           dog \\
                                       &                           a dog is barking&              &               \\
  \multirow{2}{*}{3S8bTR5VAp0\_000030} &                           a cat is meowing&          cat &           dog \\
                                       &                           a dog is barking&              &               \\
\multirow{2}{*}{04\_1N\_55VFw\_000030} &                           a cat is meowing&          cat &           dog \\
                                       &                           a dog is barking&              &               \\
 \multirow{2}{*}{4le\_42J5qkU\_000012} &                           a cat is meowing&          cat &           dog \\
                                       &                           a dog is barking&              &               \\
  \multirow{2}{*}{5b04Vp0loTM\_000030} &                           a cat is meowing&          cat &           dog \\
                                       &                           a dog is barking&              &               \\
  \multirow{2}{*}{5pncSb7fxEQ\_000030} &                           a cat is meowing&          cat &           dog \\
                                       &                           a dog is barking&              &               \\
  \multirow{2}{*}{6kdiESHOO3w\_000030} &                           a cat is meowing&          cat &           dog \\
                                       &                           a dog is barking&              &               \\
  \multirow{2}{*}{6VpcBh1KPSM\_000001} &                           a cat is meowing&          cat &           dog \\
                                       &                           a dog is barking&              &               \\
  \multirow{2}{*}{7cIVRdCLnW4\_000064} &                           a cat is meowing&          cat &           dog \\
                                       &                           a dog is barking&              &               \\
  \multirow{2}{*}{JQ39VPSbQ2o\_000000} &          a race car is driving on the road&     race car &    police car \\
                                       &        a police car is driving on the road&              &               \\
  \multirow{2}{*}{M-bmsXbJBdw\_000034} &        a race car is driving on the street&     race car &    police car \\
                                       &      a police car is driving on the street&              &               \\
  \multirow{2}{*}{kJe373Z1qsc\_000050} &      a race car is driving down the street&     race car &    police car \\
                                       &    a police car is driving down the street&              &               \\
 \multirow{2}{*}{KW\_OFhShBfI\_000040} &        a race car is driving down the road&     race car &    police car \\
                                       &      a police car is driving down the road&              &               \\
 \multirow{2}{*}{LGdZx\_Ng2OU\_000070} &                      a race car is driving&     race car &    police car \\
                                       &                    a police car is driving&              &               \\
  \multirow{2}{*}{LSMgG64MW2U\_000130} &      a race car is driving down the street&     race car &    police car \\
                                       &    a police car is driving down the street&              &               \\
  \multirow{2}{*}{lVAPg1giCr8\_000010} &      a race car is driving down the street&     race car &    police car \\
                                       &    a police car is driving down the street&              &               \\
  \multirow{2}{*}{m6iAg3VoVFo\_000050} &        a race car is driving down the road&     race car &    police car \\
                                       &      a police car is driving down the road&              &               \\
  \multirow{2}{*}{MmIIjAzgw30\_000180} &        a race car is driving down the road&     race car &    police car \\
                                       &      a police car is driving down the road&              &               \\
  \multirow{2}{*}{o0CMD5nm-48\_000380} &        a race car is driving down the road&     race car &    police car \\
                                       &      a police car is driving down the road&              &               \\
  \multirow{2}{*}{2wUsyQY0R5Q\_000360} &     a boy is riding a skateboard on a ramp&   skateboard & surfboard+sea \\
                                       &     a boy is riding a surfboard on the sea&              &               \\
  \multirow{2}{*}{4yJFeZd3oYg\_000030} &     a man is riding a skateboard on a ramp&   skateboard & surfboard+sea \\
                                       &     a man is riding a surfboard on the sea&              &               \\
  \multirow{2}{*}{22b6SLUvGHk\_000020} &     a man is riding a skateboard on a ramp&   skateboard & surfboard+sea \\
                                       &     a man is riding a surfboard on the sea&              &               \\
  \multirow{2}{*}{38DktuXxeqQ\_000260} &     a man is riding a skateboard on a ramp&   skateboard & surfboard+sea \\
                                       &     a man is riding a surfboard on the sea&              &               \\
  \multirow{2}{*}{38Vg0ciQWBc\_000010} &     a man is riding a skateboard on a ramp&   skateboard & surfboard+sea \\
                                       &     a man is riding a surfboard on the sea&              &               \\
  \multirow{2}{*}{81FaBaq0t-8\_000225} &     a man is riding a skateboard on a ramp&   skateboard & surfboard+sea \\
                                       &     a man is riding a surfboard on the sea&              &               \\
  \multirow{2}{*}{1914bVcPq0k\_000030} &     a man is riding a skateboard on a ramp&   skateboard & surfboard+sea \\
                                       &     a man is riding a surfboard on the sea&              &               \\
  \multirow{2}{*}{Apr3yTPMZCY\_000458} &     a man is riding a skateboard on a ramp&   skateboard & surfboard+sea \\
                                       &     a man is riding a surfboard on the sea&              &               \\
  \multirow{2}{*}{ctJ2410j7qo\_000040} &     a man is riding a skateboard on a ramp&   skateboard & surfboard+sea \\
                                       &     a man is riding a surfboard on the sea&              &               \\
  \multirow{2}{*}{FIO-QGbT1-g\_000000} &     a man is riding a skateboard on a ramp&   skateboard & surfboard+sea \\
                                       &     a man is riding a surfboard on the sea&              &               \\
 \multirow{2}{*}{\_-R5EPaybpk\_000002} &                          a lion is roaring&         lion &           cat \\
                                       &                           a cat is meowing&              &               \\
 \multirow{2}{*}{\_Xha6m87OOs\_000060} &                          a lion is roaring&         lion &           cat \\
                                       &                           a cat is meowing&              &               \\
  \multirow{2}{*}{1-9ryaEsFc8\_000029} &                          a lion is roaring&         lion &           cat \\
                                       &                           a cat is meowing&              &               \\
  \multirow{2}{*}{2PSepowyWHE\_000003} &                          a lion is roaring&         lion &           cat \\
                                       &                           a cat is meowing&              &               \\
  \multirow{2}{*}{5ZtB9FnUIZs\_000016} &                          a lion is roaring&         lion &           cat \\
                                       &                           a cat is meowing&              &               \\
  \multirow{2}{*}{6YS3ewiOBkU\_000007} &                          a lion is roaring&         lion &           cat \\
                                       &                           a cat is meowing&              &               \\
  \multirow{2}{*}{9IIKUunyzM8\_000007} &                          a lion is roaring&         lion &           cat \\
                                       &                           a cat is meowing&              &               \\
  \multirow{2}{*}{9S4-bVB6v0Q\_000005} &                          a lion is roaring&         lion &           cat \\
                                       &                           a cat is meowing&              &               \\
  \multirow{2}{*}{bBMcsO6IeDE\_000021} &                          a lion is roaring&         lion &           cat \\
                                       &                           a cat is meowing&              &               \\
  \multirow{2}{*}{C0i90WmUMvE\_000109} &                          a lion is roaring&         lion &           cat \\
                                       &                           a cat is meowing&              &               \\
  \multirow{2}{*}{7IVwirRF3W0\_000030} &                                machine gun&  machine gun &     laser gun \\
                                       &                                  laser gun&              &               \\
  \multirow{2}{*}{8LVWNGRjD0g\_000252} &                                machine gun&  machine gun &     laser gun \\
                                       &                                  laser gun&              &               \\
  \multirow{2}{*}{35zwOkXkDt4\_000224} &                                machine gun&  machine gun &     laser gun \\
                                       &                                  laser gun&              &               \\
  \multirow{2}{*}{-ahgvCmiECM\_000030} &                                machine gun&  machine gun &     laser gun \\
                                       &                                  laser gun&              &               \\
  \multirow{2}{*}{AwW31u6wYvE\_000019} &                                machine gun&  machine gun &     laser gun \\
                                       &                                  laser gun&              &               \\
  \multirow{2}{*}{bnqsQhk2yX0\_000040} &                                machine gun&  machine gun &     laser gun \\
                                       &                                  laser gun&              &               \\
\multirow{2}{*}{C9n\_\_zk2DY8\_000061} &                                machine gun&  machine gun &     laser gun \\
                                       &                                  laser gun&              &               \\
  \multirow{2}{*}{kqfvQWAH0C0\_000130} &                                machine gun&  machine gun &     laser gun \\
                                       &                                  laser gun&              &               \\
  \multirow{2}{*}{LIUowNjRNwE\_000125} &                                machine gun&  machine gun &     laser gun \\
                                       &                                  laser gun&              &               \\
  \multirow{2}{*}{N59msUnyy1g\_000054} &                                machine gun&  machine gun &     laser gun \\
                                       &                                  laser gun&              &               \\
  \multirow{2}{*}{1nzZrX5JWyA\_000017} &                           a dog is howling&          dog &          lion \\
                                       &                          a lion is roaring&              &               \\
  \multirow{2}{*}{6CmqiGDOtmo\_000014} &                           a dog is howling&          dog &          lion \\
                                       &                          a lion is roaring&              &               \\
  \multirow{2}{*}{6WIPUATvzL4\_000001} &                           a dog is howling&          dog &          lion \\
                                       &                          a lion is roaring&              &               \\
  \multirow{2}{*}{BFBW5bEqCy0\_000018} &                           a dog is howling&          dog &          lion \\
                                       &                          a lion is roaring&              &               \\
  \multirow{2}{*}{d0V8UNE3Dtg\_000141} &                           a dog is howling&          dog &          lion \\
                                       &                          a lion is roaring&              &               \\
  \multirow{2}{*}{ESRiXGhb-Ww\_000095} &                           a dog is howling&          dog &           cat \\
                                       &                           a cat is meowing&              &               \\
  \multirow{2}{*}{fIramHEoZvg\_000017} &                           a dog is howling&          dog &           cat \\
                                       &                           a cat is meowing&              &               \\
  \multirow{2}{*}{fq2SbG-7Rtk\_000063} &                           a dog is howling&          dog &           cat \\
                                       &                           a cat is meowing&              &               \\
  \multirow{2}{*}{j3NuRPLUDhg\_000021} &                           a dog is howling&          dog &           cat \\
                                       &                           a cat is meowing&              &               \\
  \multirow{2}{*}{J4pwTPDqrKA\_000018} &                           a dog is howling&          dog &           cat \\
                                       &                           a cat is meowing&              &               \\
 \multirow{2}{*}{\_wQakQ-AC3A\_000020} &                         a bird is chirping&         bird &       seagull \\
                                       &                      a seagull is chirping&              &               \\
  \multirow{2}{*}{0C-5reSgR2w\_000020} &                         a bird is chirping&         bird &       seagull \\
                                       &                      a seagull is chirping&              &               \\
  \multirow{2}{*}{0yTG1Yrnmak\_000030} &                         a bird is chirping&         bird &       seagull \\
                                       &                      a seagull is chirping&              &               \\
  \multirow{2}{*}{1QWd2fVos8s\_000104} &                         a bird is chirping&         bird &       seagull \\
                                       &                      a seagull is chirping&              &               \\
 \multirow{2}{*}{3Wt\_ldHN6QE\_000113} &                         a bird is chirping&         bird &       seagull \\
                                       &                      a seagull is chirping&              &               \\
  \multirow{2}{*}{4Ruk56DiQj8\_000030} &                         a bird is chirping&         bird &       seagull \\
                                       &                      a seagull is chirping&              &               \\
  \multirow{2}{*}{4SUPgmqKe1s\_000053} &                         a bird is chirping&         bird &       seagull \\
                                       &                      a seagull is chirping&              &               \\
  \multirow{2}{*}{7WL9Orh7auA\_000324} &                         a bird is chirping&         bird &       seagull \\
                                       &                      a seagull is chirping&              &               \\
  \multirow{2}{*}{9bNTnSx8eFY\_000240} &                         a bird is chirping&         bird &       seagull \\
                                       &                      a seagull is chirping&              &               \\
  \multirow{2}{*}{997RTKzc39c\_000146} &                         a bird is chirping&         bird &       seagull \\
                                       &                      a seagull is chirping&              &               \\
  \multirow{2}{*}{0uOCCKQ3jQk\_000019} &                           a fox is barking&          fox &         tiger \\
                                       &                         a tiger is roaring&              &               \\
  \multirow{2}{*}{2Zir1UxVpxo\_000005} &                           a fox is barking&          fox &         tiger \\
                                       &                         a tiger is roaring&              &               \\
  \multirow{2}{*}{7h-RkocdbiM\_000016} &                           a fox is barking&          fox &         tiger \\
                                       &                         a tiger is roaring&              &               \\
  \multirow{2}{*}{dBgiqeXB7PI\_000038} &                           a fox is barking&          fox &         tiger \\
                                       &                         a tiger is roaring&              &               \\
  \multirow{2}{*}{eH6SkkHQ118\_000105} &                           a fox is barking&          fox &         tiger \\
                                       &                         a tiger is roaring&              &               \\
  \multirow{2}{*}{GQHfBnaGXu8\_000036} &                           a fox is barking&          fox &         tiger \\
                                       &                         a tiger is roaring&              &               \\
  \multirow{2}{*}{jU3mklfml-E\_000001} &                           a fox is barking&          fox &         tiger \\
                                       &                         a tiger is roaring&              &               \\
  \multirow{2}{*}{McWY8wmi1NE\_000045} &                           a fox is barking&          fox &         tiger \\
                                       &                         a tiger is roaring&              &               \\
  \multirow{2}{*}{qfSpVBLpmg8\_000140} &                           a fox is barking&          fox &         tiger \\
                                       &                         a tiger is roaring&              &               \\
  \multirow{2}{*}{qiWvQK-siSA\_000087} &                           a fox is barking&          fox &         tiger \\
                                       &                         a tiger is roaring&              &               \\
  \multirow{2}{*}{0Cvljw2Sssk\_000000} &                a man is playing basketball&   basketball &  explode bomb \\
                                       &         a man is playing an exploding bomb&              &               \\
 \multirow{2}{*}{6Jo\_tvf0qdI\_000009} &                a man is playing basketball&   basketball &  explode bomb \\
                                       &         a man is playing an exploding bomb&              &               \\
  \multirow{2}{*}{CWFnfL-5X-M\_000030} &         a young girl is playing basketball&   basketball &  explode bomb \\
                                       &  a young girl is playing an exploding bomb&              &               \\
\multirow{2}{*}{Do\_\_idgHWJM\_000490} &                a man is playing basketball&   basketball &  explode bomb \\
                                       &         a man is playing an exploding bomb&              &               \\
  \multirow{2}{*}{do8fVVvSvTQ\_000130} &          a young man is playing basketball&   basketball &  explode bomb \\
                                       &   a young man is playing an exploding bomb&              &               \\
  \multirow{2}{*}{GQJ3-6ZBsfg\_000200} &             two men are playing basketball&   basketball &  explode bomb \\
                                       &      two men are playing an exploding bomb&              &               \\
  \multirow{2}{*}{I5ECnXmzfCo\_000135} &          a young boy is playing basketball&   basketball &  explode bomb \\
                                       &   a young boy is playing an exploding bomb&              &               \\
  \multirow{2}{*}{KEeyw8lcPKs\_000000} &                a man is playing basketball&   basketball &  explode bomb \\
                                       &         a man is playing an exploding bomb&              &               \\
  \multirow{2}{*}{myBRFJP7Z2U\_000001} &                a man is playing basketball&   basketball &  explode bomb \\
                                       &         a man is playing an exploding bomb&              &               \\
  \multirow{2}{*}{SCskHem1qzo\_000060} &                a man is playing basketball&   basketball &  explode bomb \\
                                       &         a man is playing an exploding bomb&              &               \\
  \multirow{2}{*}{0aKYFdbqjHc\_000032} &         a firework lit up in the night sky&     firework &         water \\
                                       & a splash of water lit up in the night sky.&              &               \\
  \multirow{2}{*}{1W-i57MQ-zQ\_000590} &         a firework lit up in the night sky&     firework &         water \\
                                       & a splash of water lit up in the night sky.&              &               \\
 \multirow{2}{*}{2pxTI\_FzoqI\_000289} &         a firework lit up in the night sky&     firework &         water \\
                                       & a splash of water lit up in the night sky.&              &               \\
  \multirow{2}{*}{8LfRQTJAemw\_000322} &         a firework lit up in the night sky&     firework &         water \\
                                       & a splash of water lit up in the night sky.&              &               \\
 \multirow{2}{*}{41SLncI\_B04\_000066} &         a firework lit up in the night sky&     firework &         water \\
                                       & a splash of water lit up in the night sky.&              &               \\
  \multirow{2}{*}{a8fa79w2aIQ\_000023} &      a bursting firecracker is on the road&  firecracker &         water \\
                                       &           a splash of water is on the road&              &               \\
  \multirow{2}{*}{dyi5OukAmmU\_000016} &    a bursting firecracker is on the street&  firecracker &         water \\
                                       &         a splash of water is on the street&              &               \\
  \multirow{2}{*}{e6at9oqeIGw\_000086} &      a bursting firecracker is on the snow&  firecracker &         water \\
                                       &           a splash of water is on the snow&              &               \\
  \multirow{2}{*}{ehnGYrg3Vaw\_000252} &           a fire is exploding in the field&         fire &         water \\
                                       &            water is splashing in the field&              &               \\
 \multirow{2}{*}{XD1\_PR3n7xY\_000323} &         a firework lit up in the night sky&     firework &         water \\
                                       & a splash of water lit up in the night sky.&              &               \\
\end{longtable}
